# Supplementary material for: Hub-Accelerator: Fast and Exact Shortest Path Computation in Large Social Networks
Source: arXiv:1305.0507 source file (2013-05-02)
Supplement: Supplementary file 1 [file Appendix.tex]

\section{Appendix}
\label{apps}

\bthm
The  optimal hub-set selection problem is NP-hard and it is also equivalent to the $k$-landmark-cover problem~\cite{Potamias09}. 
\ethm

\bproof
Let us use $\mathcal{H}$ to denote the solution of optimal hub-set selection problem and $C(\mathcal{H})$ is the set of vertex pairs covered by hub-set $\mathcal{H}$.
Similarly, we use $L$ to represent the solution of $k$-landmark-cover problem and the set of vertex pairs can be covered by $L$ is denoted as $C(L)$.
Also, $|\mathcal{H}|=|L|=k$.
We want to show that $|C(\mathcal{H})| = |C(L)|$. 

Firstly, we prove that $|C(L)| \ge |C(\mathcal{H})|$. 
%For any vertex pair $(s,t) \in C(\mathcal{H})$, we know that $d(s,t)=min_{x \in L_H(s) \wedge y \in L_H(t)} (d(s,x)+d(x,y)+d(y,t))$.
For any vertex pair $(s,t) \in C(\mathcal{H})$, there are two vertices $x \in L_H(s)$ and $y \in L_H(t)$ such that $d(s,t)=d(s,x)+d(x,y)+d(y,t)$.
If we select all vertices in $\mathcal{H}$ as landmarks $L^\prime$ (i.e., $L^\prime=\mathcal{H}$), 
vertex pair $(s,t)$ is guaranteed to be covered by $L^\prime$, such that $d(s,t)=d(s,x)+d(x,t)$ because $x \in L_H(s) \subseteq \mathcal{H} = L^\prime$.
Therefore, any vertex pair belonging to $C(\mathcal{H})$ can be covered by traditional landmark approach using $\mathcal{H}$ as landmarks.
In other words, $\mathcal{H}$ is a feasible solution for $k$-landmark-cover problem, thus $|C(L)| \ge |C(\mathcal{H})|$.   

Secondly, we prove that $|C(\mathcal{H})| \ge |C(L)|$.
According to the proof of lemma~\ref{goodcorepath}, if $SP(s,t)$ is one shortest path for vertex pair $(s,t) \in C(L)$,  
we always are able to generate another path $P(s,t)$ using landmarks $L$ as hub-set such that $|P(s,t)| \le |SP(s,t)|$.
Since $SP(s,t)$ is shortest path, $P(s,t)$ is also shorest path, thus $(s,t)$ is covered by hub-set $L$.
Therefore, any vertex pair covered by $L$ can be covered by hub-set comprising of all vertices in $L$.
As $\mathcal{H}$ with $k$ vertices is able to cover maximal number of vertex pairs, 
we claim that $|C(\mathcal{H})| \ge |C(L)|$.

Putting both together, the lemma holds.

\eproof

\comment{
Following the similar idea in the proof of lemma~\ref{equal}, our optimal $K$ core landmark selection problem is also equivalent to $Landmark_d$ problem in~\cite{Potamias:2009:FSP:1645953.1646063}, which is still NP-hard.
In this case, we need to select landmarks in a more practical and efficient manner for massive social networks.

\bdefin{\bf (Optimal Core Landmark Selection Problem)}
Given an unweighted and directed graph $G=(V,E)$, optimal landmark selection problem tries to find minimum number of landmarks $L \in V$,
such that $L$ is able to cover any reachable vertex pair $(s,t) \in V \times V$.
\edefin

We build an interesting connections between optimal core landmark selection problem and landmark-cover problem stated in~\cite{Potamias:2009:FSP:1645953.1646063}, which aims at finding a minimum number landmarks to recover any vertex pair using traditional landmark indices.

\blemma
\label{equal}
Optimal core landmark selection problem is equivalent to landmark-cover problem~\cite{Potamias:2009:FSP:1645953.1646063}.
\elemma
\bproof
Let us use $L$ to denote the optimal solution for landmark cover problem, and use $L_H$ to the solution for optimal core landmark selection problem.
On the one hand, given landmarks $L_H$, for any vertex pair $(s,t)$, if we can find two landmarks $x,y \in L_H$ to cover it (i.e., $d(s,t)=d(s,x)+d(x,y)+d(y,t)$, $x \in L_{H}(s)$ and $y \in L_{H}(t)$),
we are also able to restore their distance using one of landmarks based on traditional indexing scheme (i.e., $d(s,t)=d(s,x)+d(x,t)$ and $x \in L(s)$).
In other words, $L_H$ is a feasible solution for landmark cover problem.
Therefore, $|L_H| \ge |L|$.

On the other hand, given landmarks $L$, according to lemma~\ref{goodcorepath},
we are able to assign each vertex $u$ indices $L_{H}(u) \subseteq L$.
These core landmark indices are sufficient to recover shortest paths of all vertex pairs that can be recovered by $L$ based on traditional landmark indexing scheme.
Therefore, $\cup_{u \in V \setminus L} L_{H}(u)  \subseteq L$ is a feasible solution for optimal core landmark selection problem.
Moreover, since $L_H$ is optimal solution, meaning $|\cup_{u \in V \setminus L} L_{H}(u)| \ge |L_H|$,
thus $|L_H| \le |L|$.

Putting both together, we have $|L|=|L_H|$ following the statement in the lemma.
\eproof

Since landmark cover problem~\cite{Potamias:2009:FSP:1645953.1646063} has been proved to be NP-hard, we easily establish following result:

\blemma
Optimal core landmark selection problem is NP-hard.
\elemma
}

\comment{
Major problems related to six-degree shortest path query:
\begin{enumerate}
  \item finding shortest path with length $5$ or $6$ is most expensive;
  \item the shortest path involving hub node (with very high vertex degree) should be considered separately;
\end{enumerate}

Focussing on SP with length $5$ and $6$, possible solution and related subproblems:
\noindent 1) straightforward method: bidirectional BFS (expanding from source and destination at most $3$ steps). 
This method is rather time consuming, especially the number of vertices with $3$-step away can be up to several millions when average vertex degree is around $100$.

\noindent 2) bidirectional BFS (expanding from source and destination in $2$ steps). Assuming $L_2(s)$ and $L_2(t)$ are the vertices which are $2$-step away from source and destination, respectively.
The remaining problems are 
\begin{enumerate}
  \item how to efficiently check the adjacency of vertices between $L_2(s)$ and $L_2(t)$ for SP with length $5$?
        how to efficiently check find one common neighbor between $L_2(s)$ and $L_2(t)$ for SP with length $6$?
  \item can we utilize 2-hop idea to reduce cost?
  \item other methods?
  \item assuming vertex degree follows power law distribution, how to estimate the number of hub node?
    $p(x)=x^{-\gamma}$, $P(X>k)=\int_k^{d_{max}} x^{-\gamma} dx = \frac{1}{1-\gamma} x^{-\gamma+1} \mid_k^{d_{max}} $
\end{enumerate}

\noindent 3) For hub node, the basic idea is to materialize some information to avoid the expansion from hub node (since even $2$-expansion is too impractical for hub node)
\begin{enumerate}
  \item for query $(s,t)$, assuming $s$ is hub node, we wish to guarantee that at least one of vertices $u$ in $t$'s $2$-step expansion ball is marked as intermediate leading to the shortest path?
    Also, $u$'s consecutive node within shortest path $SP_{s,t}$ should be recorded for guiding direction.
  \item do we need to materialize every pair of hub nodes' shortest path? 
  \item how to incorporate hub node into our above bidirectional search? 
\end{enumerate}

\noindent 4) another idea is to utilize gate graph to reduce search space.
\begin{enumerate}
  \item given gate graph, what is search rule for each query (such as categorize each gate vertex's neighbors into $1$-neighbors or $2$-neighbors (edge weight is $2$)? 
  how to perform bidirectional search for SP with length from $3$ to $6$? The detailed study would show the benefit of this method compared to traditional one.
  \item check adjacency and common neighbor in gate graph
  \item what is the optimality criteria for gate-vertex set (or gate graph)? For instance, minimize gate-vertex set? minimize the number of edges in gate graph? minimize $\sum_{v \in V} L(v)$ where $L(v)$ is the number of gate vertices assigned to each vertex $v$?
    The ratio of the size of gate vertices within 2-step expansion and its $2$-step neighbors $\frac{N^\ast_2(v)}{N_2(v)}$?
  \item how to handle hub node in this framework? what is the relationship between gate vertex and hub node?
  \item approximate $6$-degree SP? If $d(s,t)\le 6$, one path with length no greater than $6$ is return (not necessarily shortest path)?
\end{enumerate}
}
